# Supplementary material for: Origins of Very Low Helium Abundance Streams Detected in the Solar Wind Plasma
Source: arXiv:2410.04713 source file (2024-10-07)
Supplement: Supplementary file 1 [file Supplementary_Tables_low_AHe.pdf]

*Supplementary Table 1: The low helium abundance events ($A_{He}$ <1%) observed by WIND and PSP spacecrafts are shown below. The duration of events observed by WIND is greater than 48 hours. The PSP events are of shorter duration and chosen based on the 360$^o$ observations of alpha and protons in the SPAN-I instrument. The start and end times, duration, average $A_{He}$, $N_p$, $N_a$, Average velocities of alphas and protons, proton temperature, alpha temperature and velocity difference between alphas and protons are shown for Wind and PSP events. $O^{7+}/O^{6+}$ and Fe/O (using ACE data) are shown in the case of Wind only. The majority of events show higher proton number density (Np) compared to the average value of Np over the two SCs (6.29), while the densities of alpha particles are decreased. In addition, the velocity difference is almost zero in WIND events, whereas the PSP event shows a finite difference between the alpha and proton velocities. The proton and alpha temperatures are low for these events.*

| WIND EVENTS | | | | | | | | | | | | | | |
|---|---|---|---|---|---|---|---|---|---|---|---|---|---|---|
| | Start time | | End time | | Duration Hours | Average $A_{He}$ | Average Np (6.29) | Average Na (0.19) | Average Velocity (p) | Average Velocity (He) | Proton Temperature | Alpha Temperature | V(p)-V(He) | O7+/O6+ | Fe/O |
| | Date | Time | date | Time | | | | | | | | | | | |
| 1 | 1995-07-01 | 20:30:00 | 1995-07-03 | 21:30:00 | 49 | 0.54±0.24 | 14.38±4.95 | 0.082±0.047 | 341.74±12.11 | 340.49±11.56 | 34048.4 | 77149.7 | 0.14 | nan | nan |
| 2 | 1996-04-06 | 15:30:00 | 1996-04-08 | 17:30:00 | 50 | 0.41±0.29 | 14.41±5.73 | 0.061±0.047 | 309.23±13.95 | 308.06±13.67 | 16228.1 | 43921.1 | 0.51 | nan | nan |
| 3 | 2006-10-18 | 00:30:00 | 2006-10-20 | 02:30:00 | 50 | 0.63±0.43 | 11.87±4.79 | 0.068±0.040 | 322.76±17.49 | 321.55±17.38 | 17024.2 | 18704.9 | 1.36 | 0.23 | 0.18 |
| 4 | 2007-03-20 | 16:30:00 | 2007-03-23 | 08:30:00 | 64 | 0.40±0.18 | 11.41±3.17 | 0.045±0.025 | 285.48±18.70 | 284.78±17.94 | 17510.5 | 25856.4 | 1.23 | 0.174 | 0.22 |
| 5 | 2007-09-11 | 05:30:00 | 2007-09-13 | 11:30:00 | 54 | 0.46±0.19 | 7.31 ±1.74 | 0.031±0.011 | 286.20±14.68 | 287.92±15.97 | 10924.8 | 14344.5 | 0.69 | 0.098 | 0.38 |
| 6 | 2007-10-09 | 21:30:00 | 2007-10-12 | 10:30:00 | 61 | 0.45±0.31 | 11.25±4.66 | 0.048±0.043 | 271.79±9.53 | 273.69±13.16 | 11538.3 | 10332.2 | 2.64 | 0.17 | 0.16 |
| 7 | 2007-11-05 | 18:30:00 | 2007-11-08 | 02:30:00 | 56 | 0.42±0.25 | 10.66±1.28 | 0.044±0.029 | 268.05±12.92 | 271.08±12.29 | 13173.1 | 16152.5 | -0.81 | 0.192 | 0.17 |
| 8 | 2008-09-12 | 21:30:00 | 2008-09-14 | 23:30:00 | 50 | 0.44±0.39 | 11.55±7.55 | 0.062±0.097 | 308.79±21.38 | 307.70±21.82 | 20149 | 47918.9 | 0.72 | 0.147 | 0.24 |
| 9 | 2008-11-12 | 03:30:00 | 2008-11-15 | 06:30:00 | 75 | 0.47±0.13 | 6.99 ±2.15 | 0.035±0.011 | 311.55±17.70 | 308.94±19.45 | 22780.4 | nan | 0.5 | 0.098 | 0.18 |
| 10 | 2009-02-06 | 11:30:00 | 2009-02-08 | 12:30:00 | 49 | 0.52±0.21 | 7.93 ±2.16 | 0.041±0.015 | 314.06±7.87 | 312.02±7.85 | 20728.9 | 21348.1 | 1.2 | 0.084 | 0.16 |
| 11 | 2009-08-15 | 00:30:00 | 2009-08-17 | 21:30:00 | 69 | 0.47±0.21 | 8.09 ±3.16 | 0.042±0.022 | 283.92±11.51 | 282.51±13.06 | 17609.9 | nan | 2.17 | 0.203 | 0.29 |
| 12 | 2009-11-10 | 02:30:00 | 2009-11-12 | 04:30:00 | 50 | 0.68±0.25 | 5.45 ±0.86 | 0.036±0.009 | 322.96±28.08 | 320.31±29.99 | 23808.7 | 12472.8 | -1.09 | 0.058 | 0.18 |
| 13 | 2009-12-08 | 13:30:00 | 2009-12-11 | 00:30:00 | 59 | 0.66±0.18 | 7.20 ±0.98 | 0.046±0.013 | 292.19±13.51 | 292.88±13.97 | 20989.4 | 20091.7 | -0.22 | 0.053 | 0.22 |
| 14 | 2010-08-11 | 04:30:00 | 2010-08-13 | 05:30:00 | 49 | 0.55±0.17 | 6.16 ±2.15 | 0.031±0.006 | 385.04±52.11 | 385.77±52.42 | 35160.6 | nan | -2.19 | 0.187 | 0.19 |

| | | | | | | | | | | | | | | |
|---|---|---|---|---|---|---|---|---|---|---|---|---|---|---|
| 15 | 2017-06-08 | 18:30:00 | 2017-06-11 | 15:30:00 | 69 | 0.54±0.26 | 12.62±5.41 | 0.067±0.036 | 301.55±18.32 | 299.59±17.69 | 18581.2 | 17544.5 | 0.54 | 0.222 | 0.29 |
| 16 | 2018-01-06 | 02:30:00 | 2018-01-08 | 09:30:00 | 55 | 0.50±0.29 | 14.82±9.09 | 0.091±0.131 | 298.42±15.81 | 297.16±15.73 | 19311.1 | 35658.2 | 1.62 | 0.251 | 0.18 |
| 17 | 2018-06-15 | 20:30:00 | 2018-06-17 | 22:30:00 | 50 | 0.52±0.30 | 11.81±6.25 | 0.066±0.085 | 305.67±9.98 | 304.63±10.40 | 20821.3 | 56401 | 2.34 | 0.149 | 0.32 |
| 18 | 2018-10-19 | 09:30:00 | 2018-10-21 | 12:30:00 | 51 | 0.48±0.27 | 11.42±6.29 | 0.052±0.044 | 302.50±11.52 | 300.54±11.85 | 20801.6 | 53313.3 | 0.75 | 0.138 | 0.28 |
| 19 | 2019-03-22 | 22:30:00 | 2019-03-25 | 01:30:00 | 51 | 0.63±0.56 | 9.69 ±6.58 | 0.070±0.103 | 279.33±17.51 | 281.45±18.02 | 17336.5 | 42725.2 | 2.63 | 0.175 | 0.38 |
| 20 | 2019-06-06 | 02:30:00 | 2019-06-08 | 18:30:00 | 64 | 0.51±0.36 | 11.91±11.44 | 0.074±0.180 | 303.38±17.22 | 302.11±17.87 | 20394 | 32727.5 | 0.17 | 0.126 | 0.31 |
| 21 | 2019-12-28 | 19:30:00 | 2019-12-31 | 19:30:00 | 72 | 0.48±0.20 | 11.98±4.55 | 0.058±0.036 | 305.79±9.51 | 304.49±10.44 | 22735.6 | 27528.1 | 0.06 | nan | nan |
| 22 | 2020-05-13 | 08:30:00 | 2020-05-15 | 10:30:00 | 50 | 0.46±0.25 | 12.39±3.56 | 0.056±0.028 | 297.73±7.28 | 297.67±7.12 | 17621.3 | 19362.8 | 1.01 | nan | nan |
| 23 | 2020-05-16 | 14:30:00 | 2020-05-18 | 22:30:00 | 56 | 0.53±0.19 | 8.65 ±1.99 | 0.048±0.022 | 307.24±11.62 | 306.31±12.62 | 25843.1 | nan | 1.23 | nan | nan |
| 24 | 2020-06-05 | 12:30:00 | 2020-06-07 | 16:30:00 | 52 | 0.60±0.27 | 11.47±5.36 | 0.075±0.074 | 319.55±12.59 | 317.76±13.08 | 31391.9 | 69127.9 | 0.28 | nan | nan |
| 25 | 2020-06-20 | 00:30:00 | 2020-06-23 | 16:30:00 | 88 | 0.48±0.22 | 8.84 ±4.10 | 0.037±0.014 | 309.10±16.78 | 304.70±16.73 | 21309.9 | 21634.2 | 1.5 | nan | nan |
| 26 | 2020-09-19 | 19:30:00 | 2020-09-21 | 22:30:00 | 51 | 0.43±0.38 | 9.88 ±3.98 | 0.048±0.053 | 294.89±11.06 | 296.61±10.31 | 16079.7 | 189721 | 0.75 | nan | nan |
| 27 | 2020-10-13 | 18:30:00 | 2020-10-16 | 10:30:00 | 64 | 0.47±0.24 | 10.73±3.67 | 0.050±0.026 | 284.84±13.49 | 285.23±13.33 | 18221.9 | 25273.6 | 1.27 | nan | nan |
| 28 | 2021-08-22 | 21:30:00 | 2021-08-24 | 22:30:00 | 49 | 0.64±0.90 | 13.03±3.11 | 0.085±0.110 | 305.92±12.43 | 304.51±13.10 | 25252.6 | 60986.2 | 2.36 | nan | nan |

PSP Events

| | Start time | | End time | | Duration Hours | Average $A_{He}$ | Average Np | Average Na | Average Velocity (p) | Average Velocity (He) | Proton Temp | Alpha Temp | V(p)-V(He) |
|---|---|---|---|---|---|---|---|---|---|---|---|---|---|
| | Date | Time | date | Time | | | | | | | | | |
| 1 | 2020-01-28 | 00:00:00 | 2020-01-28 | 05:30:00 | 5.5 | 0.74 | 157.18±41.23 | 1.05±0.26 | 529.79±36.89 | 418.84±45.54 | 730288.43 | 6285990.00 | 110.95 |
| 2 | 2020-01-28 | 20:00:00 | 2020-01-29 | 02:00:00 | 6 | 0.27 | 398.55±73.73 | 1.04±0.19 | 327.07±29.42 | 395.44±32.57 | 480635.34 | 4034057.67 | 68.37 |
| 3 | 2021-08-09 | 00:00:00 | 2021-08-09 | 11:00:00 | 11 | 0.94 | 2968.65±798.08 | 27.76±10.29 | 289.16±31.73 | 325.64±49.72 | 408999.30 | 2446157.92 | 36.47 |
| 4 | 2022-02-24 | 08:30:00 | 2022-02-24 | 16:00:00 | 7.5 | 0.84 | 1605.35±370.90 | 12.92±2.88 | 367.23±39.50 | 443.35±48.58 | 577080.97 | 4295912.54 | 76.12 |

*Supplementary Table 2: The solar wind sources of the events shown in the supplementary table are presented. The match between the model output and observed solar wind is shown in column 2. The solar wind start and end times estimated by the model are presented in columns 2 and 3. The outputs of the model, i.e., distance from the current sheet, the magnetic field at the foot points, longitude of foot points, distance from coronal holes and expansion factors, are shown in the rest of the columns.*

| Event Number | Model Reliable | Model Start time | | Model end time | | Current sheet distance | B foot point (magnitude) | Lon foot point | Coronal hole distance | Expansion factor |
|---|---|---|---|---|---|---|---|---|---|---|
| | | | | | | Deg | G | Deg (1Rs) | Deg | ## |
| 1 | No | | | | | | | | | |
| 2 | No | | | | | | | | | |
| 3 | No | | | | | | | | | |
| 4 | Yes | 2007-03-21 | 01:32:44 | 2007-03-23 | 08:04:59 | 8.3±1.4 | 3.1±1.2 | 207.6±5.6 | 1.7±0.4 | 12.1±6.5 |
| 5 | Yes | 2007-09-11 | 03:47:22 | 2007-09-13 | 11:40:59 | 8.7±5.3 | 6.7±2.7 | 33.7±14.1 | 1.9±0.4 | 40.9±15.6 |
| 6 | Yes | 2007-10-10 | 00:47:48 | 2007-10-12 | 11:55:14 | 3.1±2.0 | 4.7±1.5 | 95.2±129.2 | 1.5±0.5 | 61.9±78.8 |
| 7 | No | | | | | | | | | |
| 8 | Yes | 2008-09-12 | 23:29:45 | 2008-09-15 | 05:19:06 | 5.7±2.6 | 2.4±1.3 | 225.4±5.7 | 2.8±0.9 | 13.6±12.6 |
| 9 | Yes | 2008-11-12 | 18:10:56 | 2008-11-15 | 13:58:48 | 5.1±1.3 | 3.4±1.3 | 164.2±4.8 | 2.0±0.5 | 15±7.6 |
| 10 | Yes | 2009-02-06 | 11:39:50 | 2009-02-08 | 22:12:17 | 6±0.4 | 5.2±1.6 | 108.2±2.6 | 2.2±0.2 | 24.7±6.6 |
| 11 | Yes | 2009-08-14 | 23:50:21 | 2009-08-17 | 00:33:50 | 2±1.1 | 1.7±0.7 | 98.1±13.7 | 2.0±0.7 | 14.8±15.7 |
| 12 | Yes | 2009-11-10 | 17:14:47 | 2009-11-12 | 02:47:28 | 0.7±0.8 | 2.0±0.7 | 72.8±7.1 | 1.6±0.2 | 32.9±26.9 |
| 13 | Yes | 2009-12-08 | 12:34:50 | 2009-12-11 | 00:27:47 | 0.8±0.5 | 5.8±2.3 | 42.4±16.0 | 1.4±0.4 | 97.7±100.5 |
| 14 | Yes | 2010-08-11 | 09:53:34 | 2010-08-13 | 00:44:03 | 22.2±5.5 | 5.3±2.8 | 28.3±7.9 | 2.7±0.4 | 13.4±7.5 |
| 15 | Yes | 2017-06-08 | 20:11:45 | 2017-06-11 | 16:33:53 | 1.2±0.9 | 8.6±1.4 | 246.4±9.3 | 1.7±0.4 | 64.0±7.4 |
| 16 | No | | | | | | | | | |
| 17 | No | | | | | | | | | |
| 18 | Yes | 2018-10-19 | 07:50:52 | 2018-10-21 | 14:19:23 | 2.7±0.7 | 5.2±2.4 | 170.4±6.8 | 1.6±0.2 | 21.8±11.2 |
| 19 | No | | | | | | | | | |
| 20 | Yes | 2019-06-06 | 06:01:17 | 2019-06-07 | 21:07:11 | 6.6±0.6 | 5.4±1.1 | 349.5±6.2 | 1.8±0.3 | 18.4±3.1 |
| 21 | Yes | 2019-12-28 | 23:18:05 | 2019-12-31 | 21:47:05 | 1.5±0.7 | 4.7±1.5 | 169.6±12 | 1.3±0.4 | 64.2±94.2 |
| 22 | Yes | 2020-05-13 | 05:02:23 | 2020-05-15 | 07:58:04 | 1.1±0.3 | 4.3±0.6 | 185.3±8.4 | 1.5±0.4 | 24.2±10.1 |
| 23 | Yes | 2020-05-16 | 20:15:47 | 2020-05-18 | 22:19:20 | 1.05±0.1 | 6.2±1.5 | 115.6±6.3 | 1.6±0.5 | 51.2±12.1 |
| 24 | Yes | 2020-06-05 | 15:53:25 | 2020-06-07 | 13:32:35 | 1.9±0.9 | 3.3±1.6 | 213.8±5.1 | 2.5±0.7 | 12.2±7.2 |
| 25 | Yes | 2020-06-19 | 21:40:45 | 2020-06-23 | 05:29:28 | 2.3±0.8 | 3.9±1.1 | 25.1±7.4 | 2.4±0.7 | 14.6±3.2 |
| 26 | Yes | 2020-09-19 | 18:33:50 | 2020-09-21 | 21:53:25 | 1.2±0.001 | 7.0±3.9 | 265±9.8 | 1.5±0.3 | 166±117.2 |
| 27 | Yes | 2020-10-14 | 00:56:09 | 2020-10-16 | 09:21:53 | 1.7±0.02 | 4.2±1.8 | 303.3±10.2 | 1.4±0.4 | 17.9±7.5 |
| 28 | Yes | 2021-08-22 | 20:36:05 | 2021-08-24 | 20:59:42 | 2±1.1 | 8.0±2.7 | 113.5±27.8 | 1.4±0.6 | 62.1±15.4 |

| PSP Events | | | | | | | | | | |
|---|---|---|---|---|---|---|---|---|---|---|
| Event Number | Model Reliable | Model Start time | | Model end time | | Current sheet distance | B foot point | Lon foot point | Coronal hole distance | Expansion factor |
| | | | | | | Deg | G | Deg (1Rs) | Deg | ## |
| 1 | Yes | 2020-01-27 | 22:55:37 | 2020-01-28 | 06:29:57 | 1.3±0.2 | 1.9±0.4 | 70.2±0.6 | 1.0±0.2 | 13.9±2.9 |
| 1 | Yes | 2020-01-28 | 18:45:56 | 2020-01-29 | 03:44:29 | 2.7±0.4 | 6.1±1.0 | 58.2±0.8 | 2.7±0.01 | 23.8±3.8 |
| 1 | Yes* | 2021-08-09 | 12:42:11.00 | 2021-08-09 | 12:42:11 | 13.4±3.9 | 63.8±9.8 | 53.1±0.6 | 1.9±0.5 | 141.1±43.9 |
| 1 | No | 2022-02-24 | 14:22:33.00 | 2022-02-24 | 14:22:33 | | | | | |

* The model outputs matched the data, but the source was on the far side of the sun.

*Supplementary Table 3: - The table below displays the dominant periods calculated using the FFT and Lomb-Scargle periodogram. The top 5 periods with the maximum power are listed, with the condition that the power of these periods exceeds both the False Alarm Level and Fisher's Level. It is evident from the table that a period of approximately 2000 seconds is consistently present in almost all the events.*

| **Wind Events** | | | | | |
|---|---|---|---|---|---|
| Sr. No | Period-1 (sec) | Period-2 (sec) | Period-3 (sec) | Period-4 (sec) | Period-5 (sec) |
| 1 | 1675.48 | 1843.03 | 1275.95 | 1382.28 | 1564.84 |
| 2 | 2090.86 | 1987.61 | 2175.62 | 1769.2 | 1490.72 |
| 3 | 1640.64 | 3281.22 | 2581.96 | 2350.75 | 2019.24 |
| 4 | 2497.73 | 2103.36 | 2561.77 | 1407.19 | 1833.21 |
| 5 | 2026.15 | 1870.29 | 1736.7 | 1590.63 | 1350.77 |
| 6 | 2263.57 | 2139.2 | 2464.14 | 1908.51 | 1569.91 |
| 7 | 1546.25 | 1518.39 | 2592.91 | 1370.26 | 2160.77 |
| 8 | 2758.3 | 2456.62 | 2807.56 | 1123.04 | 2535.87 |
| 9 | 1690.8 | 3114.58 | 2545.26 | 2343.66 | 1207.72 |
| 10 | 3107.24 | 1492.72 | 1812.58 | 1903.21 | 2625.1 |
| 11 | 2011.3 | 1811.83 | 913.47 | 2170.6 | 3779.78 |
| 12 | 911.97 | 2273.28 | 1537.82 | 1651.13 | 906.7 |
| 13 | 2035.95 | 2464.57 | 1892 | 1300.76 | 1836.36 |
| 14 | 1835.53 | 1554.59 | 1291.1 | 1880.85 | 1508.41 |
| 15 | 2731.17 | 3310.49 | 3833.17 | 1883.58 | 2511.43 |
| 16 | 2437.94 | 2474.32 | 2210.4 | 1691.64 | 1246.48 |
| 17 | 2150.45 | 1682.97 | 1460.69 | 2243.95 | 3159.81 |
| 18 | 2022.78 | 2191.34 | 1325.86 | 1593.71 | 2286.61 |
| 19 | 2161.32 | 1733.81 | 1856.2 | 1972.21 | 1947.86 |
| 20 | 1513.27 | 1700.75 | 2066.49 | 2159.37 | 1941.25 |
| 21 | 2270.5 | 1576.75 | 1633.47 | 2183.18 | |
| 22 | 1776.27 | 2509.93 | 1804.03 | 1268.77 | 2748.97 |
| 23 | 1938.16 | 2269.68 | 2183.49 | 2738.01 | 1358.25 |
| 24 | 2319.94 | 2389.19 | 2078.91 | | |
| 25 | 1506.48 | 1548.55 | 1979.93 | 2410.34 | 1669.83 |
| 26 | 2085.29 | 1281.95 | 2202.76 | 2522.51 | 1221.86 |
| 27 | 1988.34 | 2101.32 | 2125.47 | 1444.66 | 2889.28 |
| 28 | 1524.07 | 1756.91 | 1946.11 | 2480.33 | 1709.43 |
| **PSP Events** | | | | | |
| 1 | 792.96 | 1524.92 | 1321.6 | 2202.67 | 3304 |
| 2 | 1966.36 | 2163 | 2403.33 | 1201.67 | 618 |
| 3 | 1982.4 | 1802.18 | 3304 | 1652 | 1723.83 |
| *4* | *600.64* | *1801.92* | *643.54* | *587.58* | *628.58* |
